# Supplementary material for: A Generalist FaceX via Learning Unified Facial Representation
Source: arXiv:2401.00551 source file (2023-12-31)
Supplement: Supplementary file 1 [file X_suppl.tex]

\clearpage
\setcounter{page}{1}
\maketitlesupplementary

%
% \section*{Overview} \label{section:app}
% In this supplementary material, we provide additional details which we could not include in the main paper due to space constraints. We present:

% % 
% \begin{itemize}
% \item more qualitative results in the wild;
% \item architecture details;
% \item data processing pipeline.
% \end{itemize}
% %

\subsection{Varied Attribute Combinations in Facial Editing}
\label{sec:task_definition}
From the standpoint of concept definition, as delineated in main paper Fig.2, the proposed facial omni-representation equation dissects a single face into a composite of distinct fine-grained attributes. The versatility of this approach is demonstrated in addressing complex facial editing tasks, wherein a judicious combination of source and target face image attributes is deployed. Simple facial attribute editing tasks necessitate the singular substitution of a specific attribute, such as hairstyle or expression, from the target with its counterpart in the source.
In tasks such as animation and inpainting, there is no need to modify the facial representation. Instead, these tasks operate on the overall image, implementing changes at the domain or pixel level.

From a practical modeling perspective, the defined face attributes can be reclassified into motion-related attributes (encompassing gaze, expression, and pose) and appearance-related attributes (comprising region-specific properties such as background, hair, facial texture, and global properties such as illumination and identity). 
Modeling motion with 3DMM parameters is straightforward. To model appearance-related attributes, we utilize a face parsing mask to extract images and features from specific local regions. This includes background, hair, and facial texture. Moreover, facial texture encompass more detailed region features such as eyebrows, glasses, nose, lips, and skin. The features from these segmented regions can be combined based on the requirements of different tasks, as illustrated in Fig. 4 of the main paper.

In comparison to prior methods that mainly rely on the combined use of appearance and structure for facial representation in editing, our approach stands out by accommodating additional editing capabilities for motion. Unlike previous techniques for reenactment, face swapping, or head swapping, our method offers flexibility in editing one or multiple attributes as needed.

\subsection{More Results In the Wild}
\label{sec:more_results}
\noindent
\textbf{Face Reenactment.}
By manipulating the parameters of the 3DMM, we gain the freedom to control motion attributes, including gaze, expression, and pose. In ~\cref{fig:facereenactwild}, this level of control extends even to unseen identities in real-world scenarios, enabling the generation of high-quality results.

\begin{figure}[h!]
	\centering
        \vspace{-1em}
	\includegraphics[width=\linewidth]{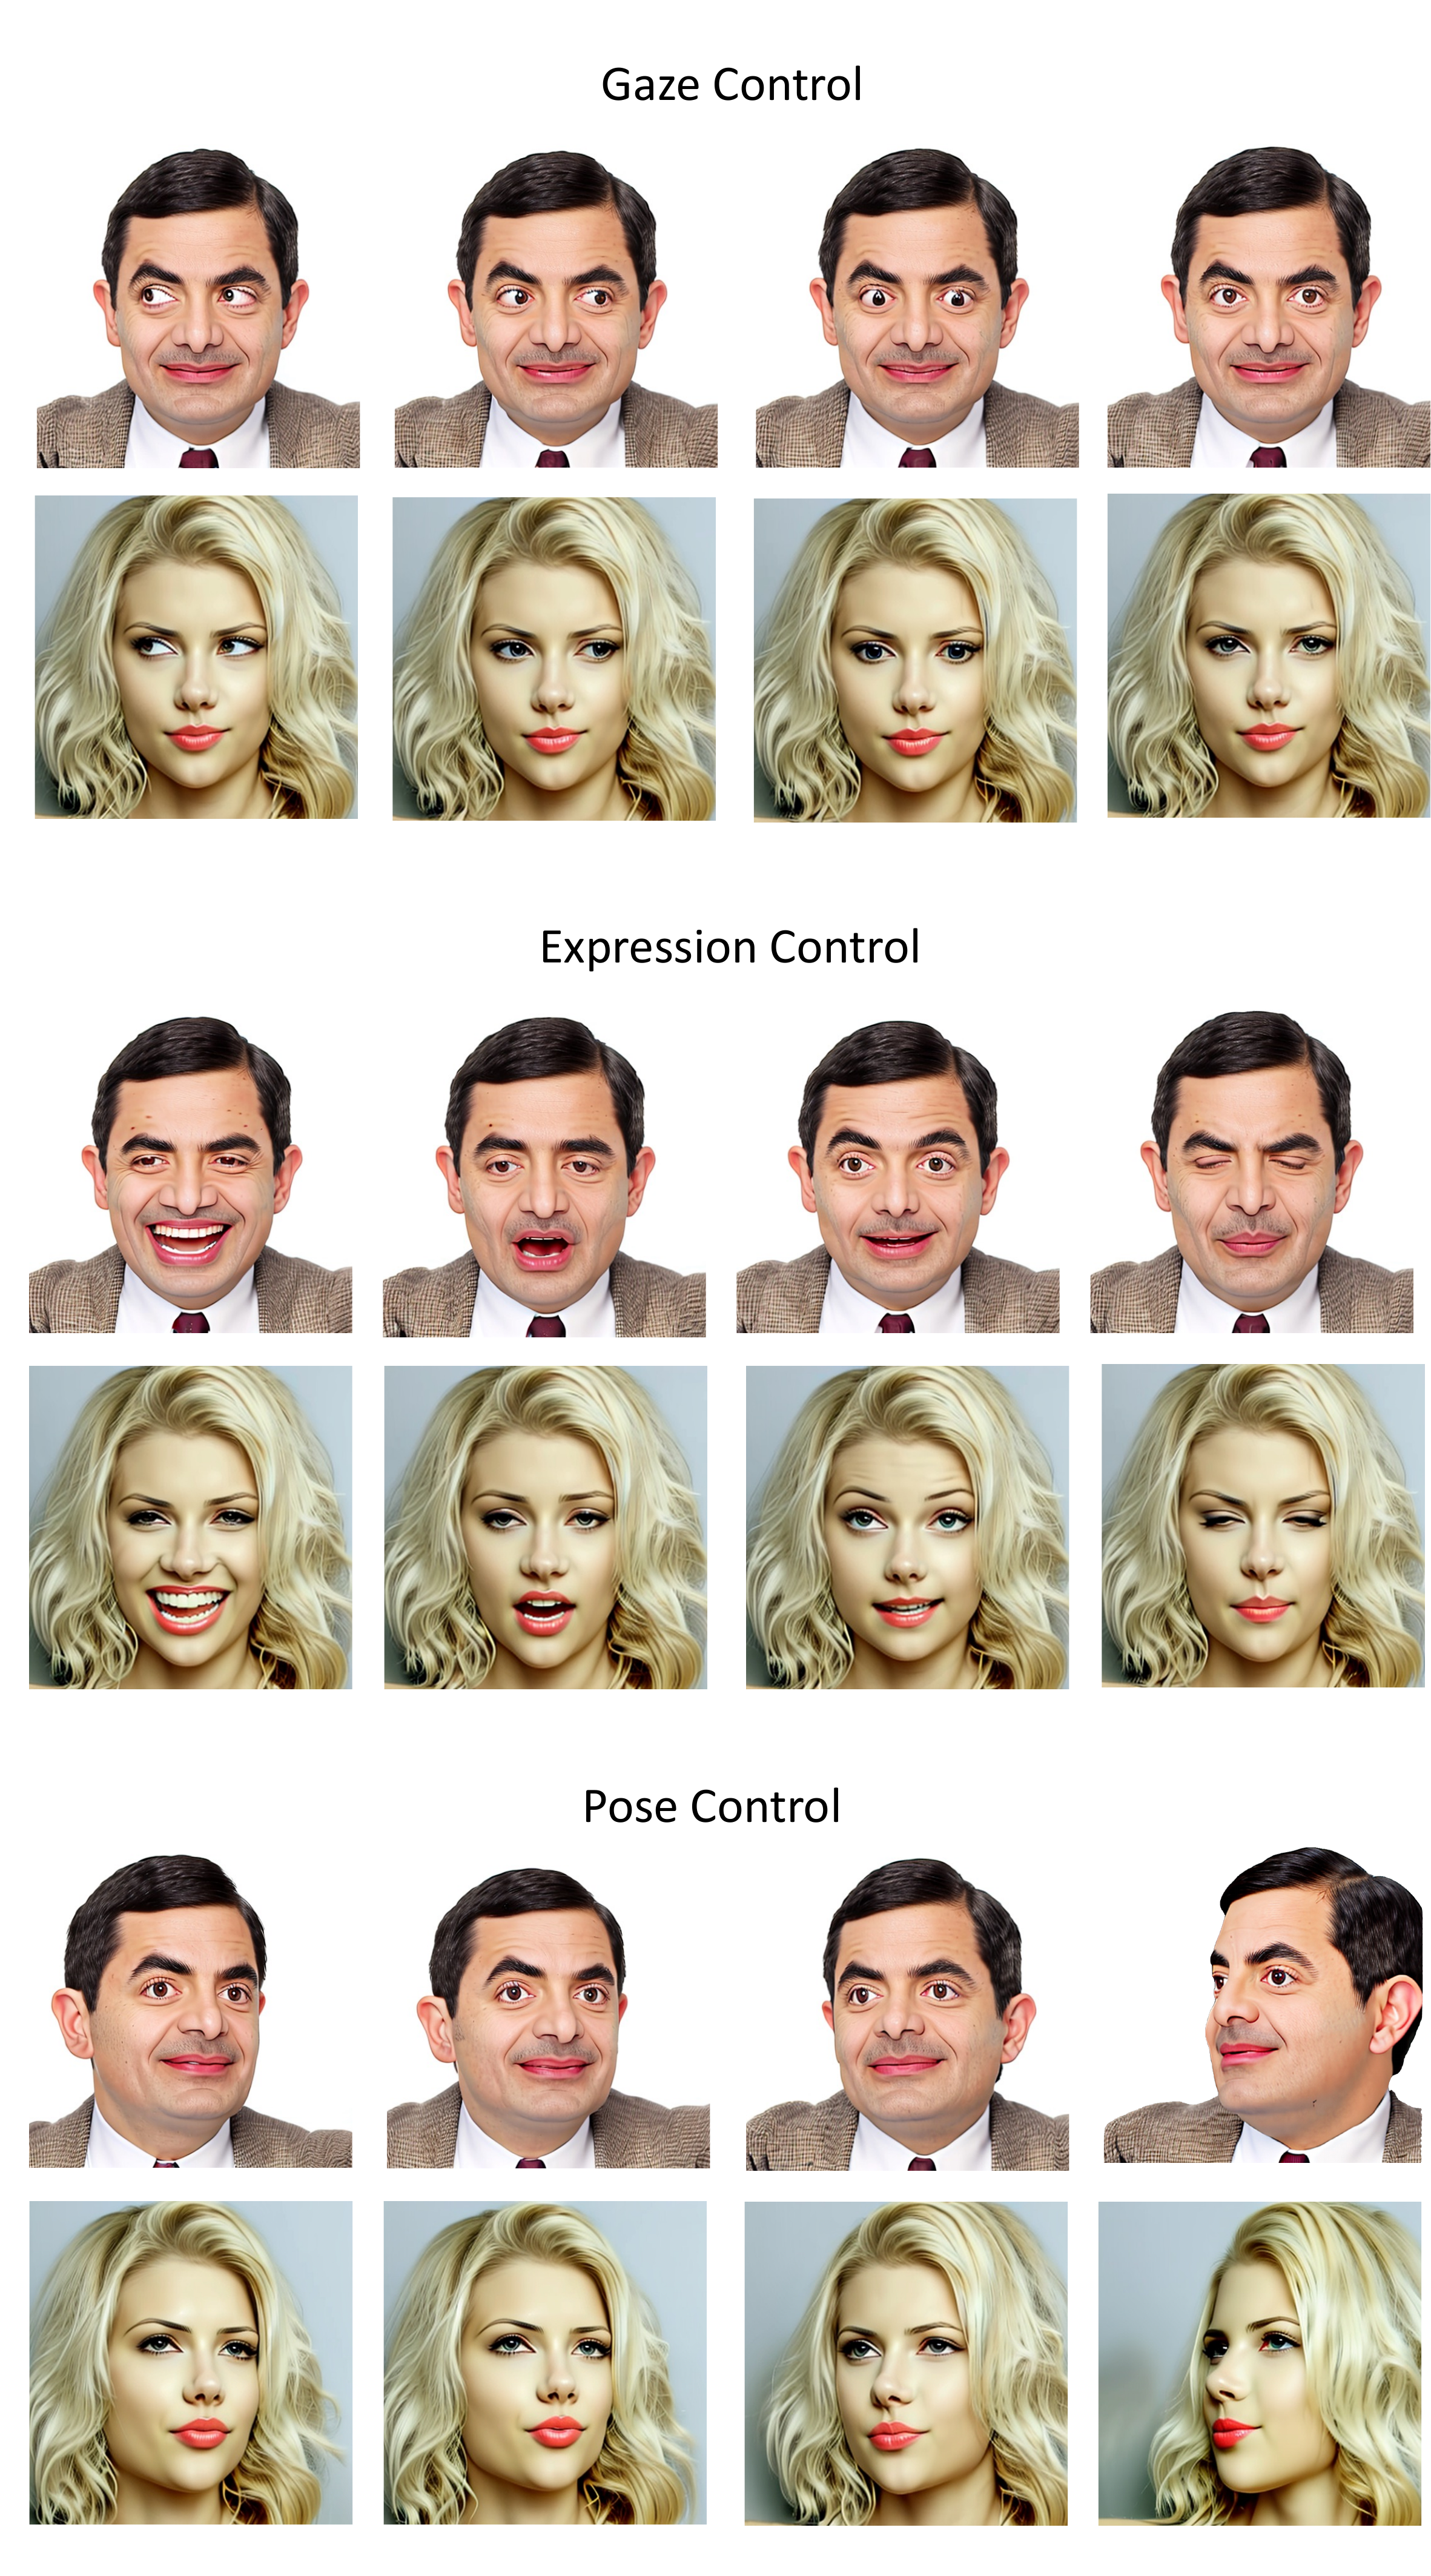}
	\vspace{-6mm}
	\caption{Face Reenactment in the wild.}
	\label{fig:facereenactwild}
	% \vspace{-1em}
\end{figure} 

\noindent
\textbf{Face Swapping.}
In ~\cref{fig:faceswapwild}, 
we select two source faces with considerable disparities in facial shape and texture to showcase the efficacy of our method. Please take note of the following key aspects:
\noindent
\textbf{\textit{1) Adaptation in facial shape:}}  Rather than merely conducting inpainting on the target face, our method dynamically swaps faces by considering the distinct facial structure of the source face.
\noindent
\textbf{\textit{2) Preservation of facial texture:}} Our approach avoids entangling skin color and texture, effectively retaining the identity features within the source face texture while simultaneously blending seamlessly with the skin tone of the target.

\noindent
\textbf{Head Swapping.}
In ~\cref{fig:headswapwild}, 
we demonstrate head-swapping results on target faces of various poses. 
The SoTA method HeSer employs a few-shot two-stage strategy (which involves reenacting the head first and then swapping it). 
In contrast, our method employs a one-shot single-stage approach. Even under extreme pose conditions, our method maintains structural plausibility, motion consistency, identity coherence, environmental appropriateness, and high generation quality.

\noindent
\textbf{Attribute Editing.}
In ~\cref{fig:mixedit}, 
We demonstrate that our method allows for simultaneous control of pose and expression while performing attribute editing, resulting in greater editing flexibility and a higher degree of freedom in attribute manipulation.

\begin{figure}[h!]
	\centering
        \vspace{-1em}
	\includegraphics[width=\linewidth]{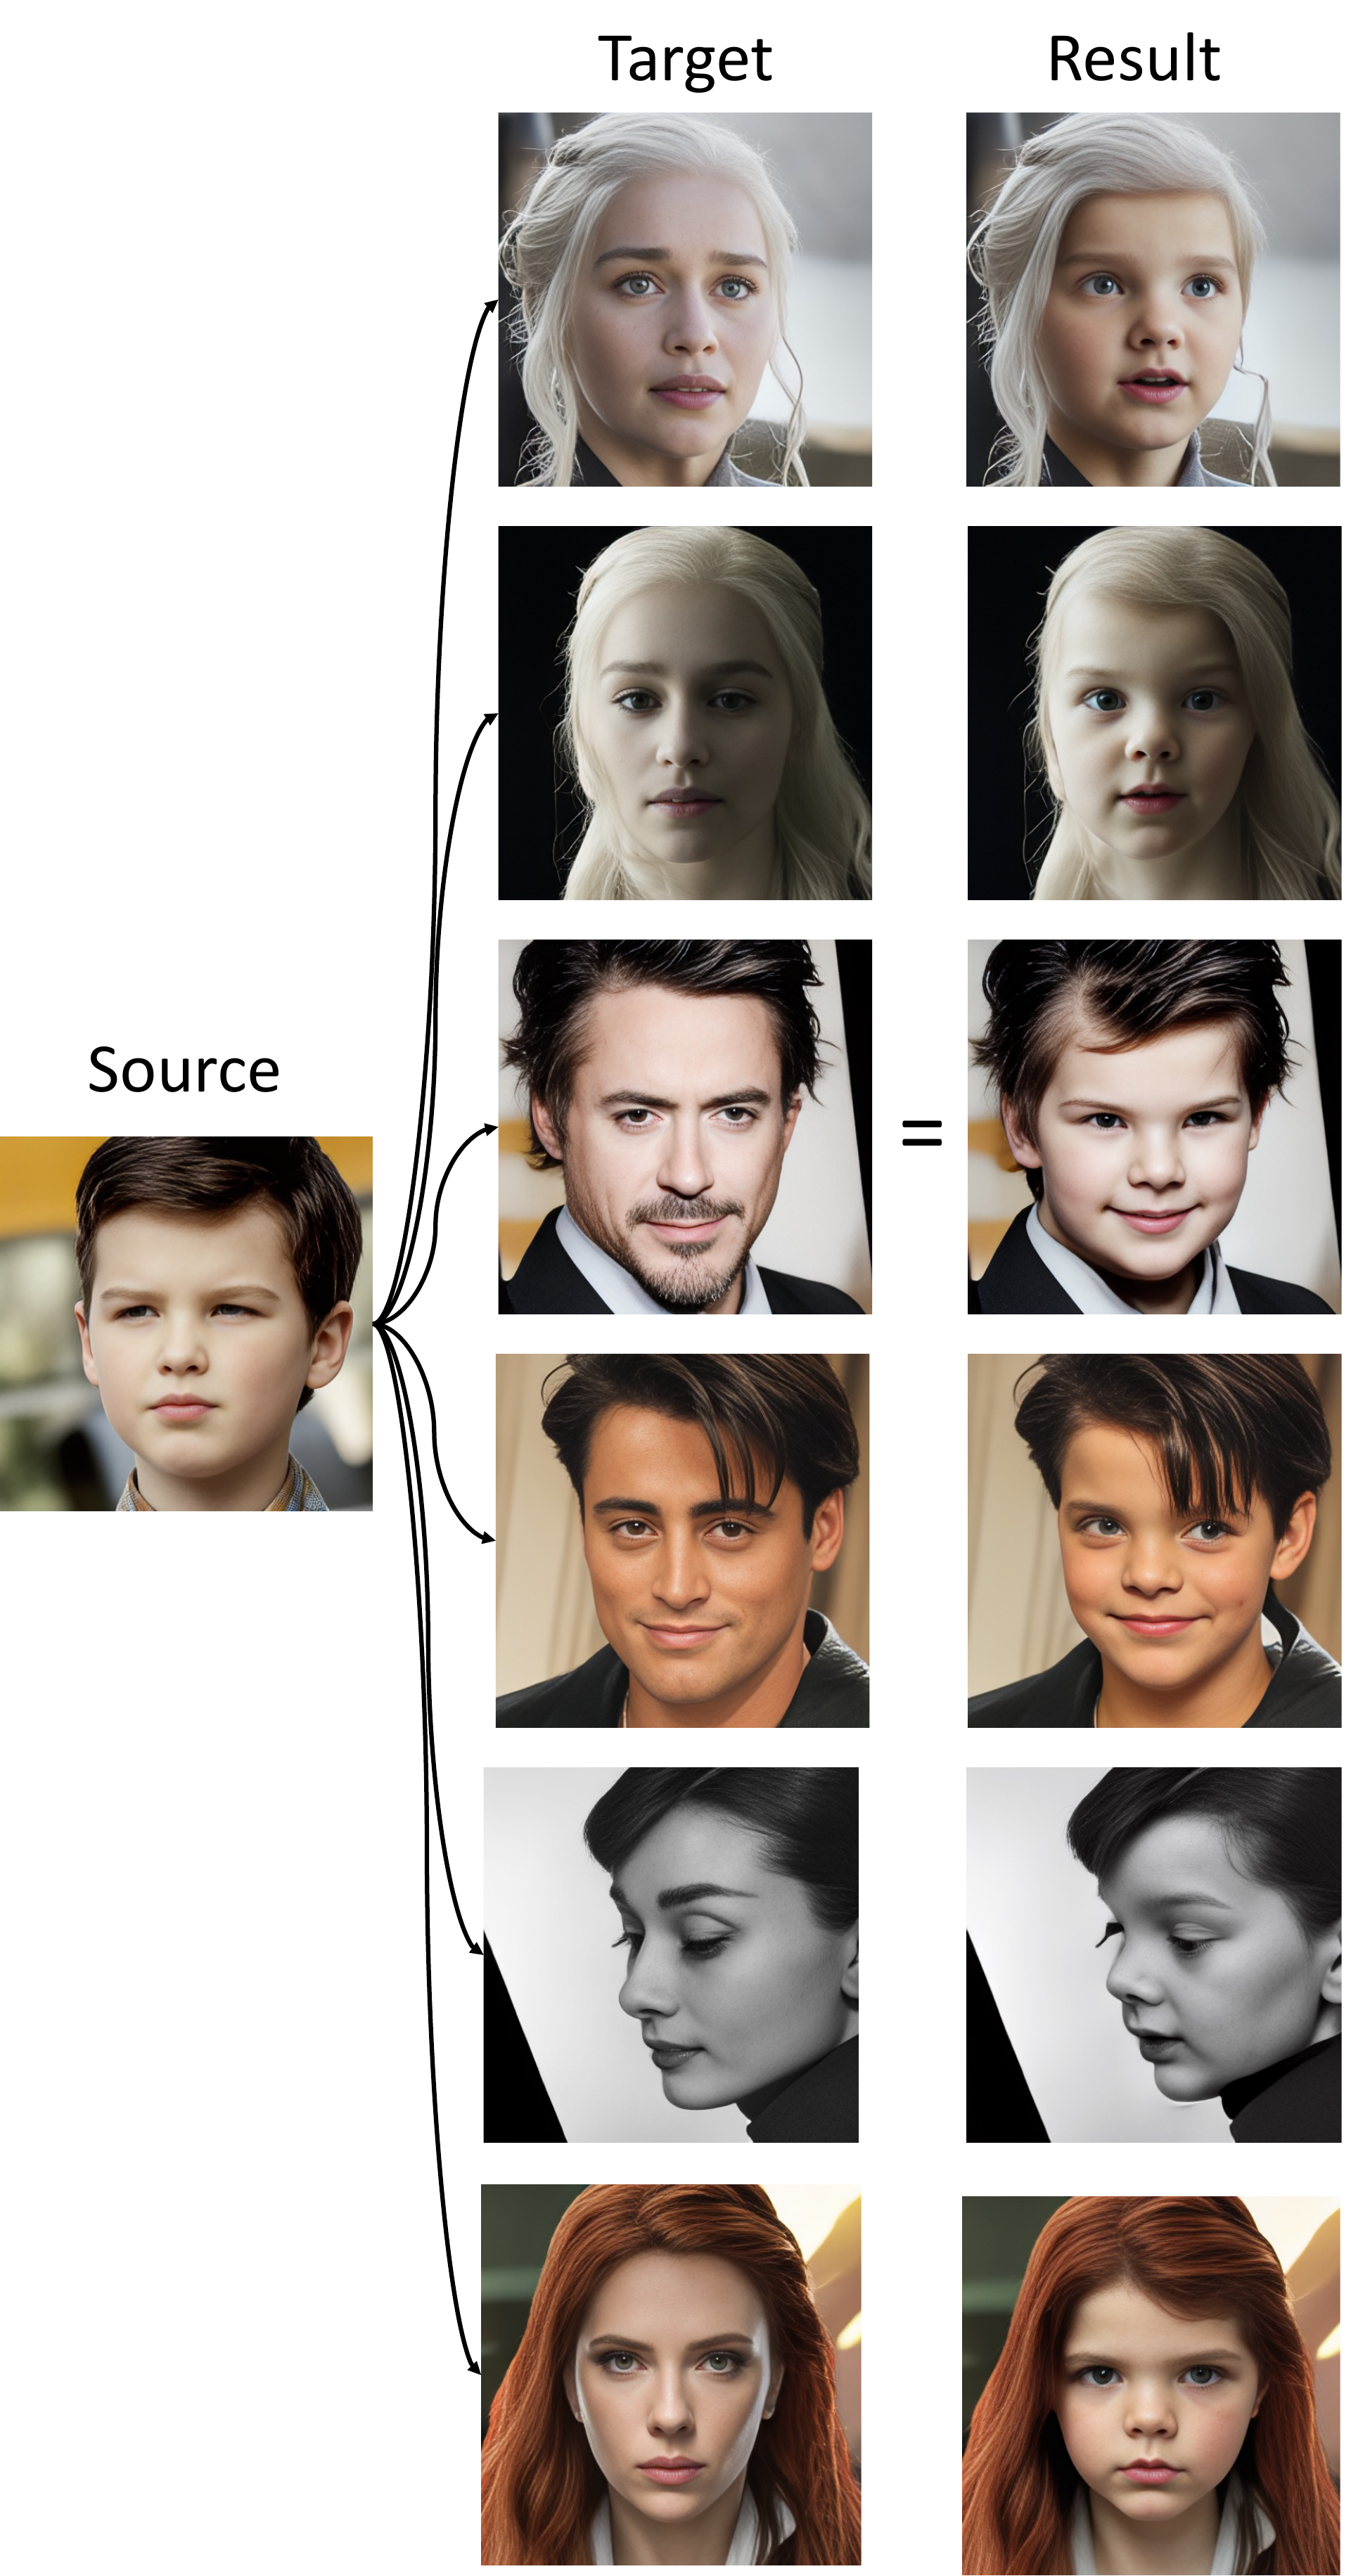}
	\vspace{-3mm}
	\caption{Face Swapping in the wild.}
	\label{fig:faceswapwild}
	% \vspace{-1em}
\end{figure} 
\begin{figure}[h!]
	\centering
	\includegraphics[width=0.97\linewidth]{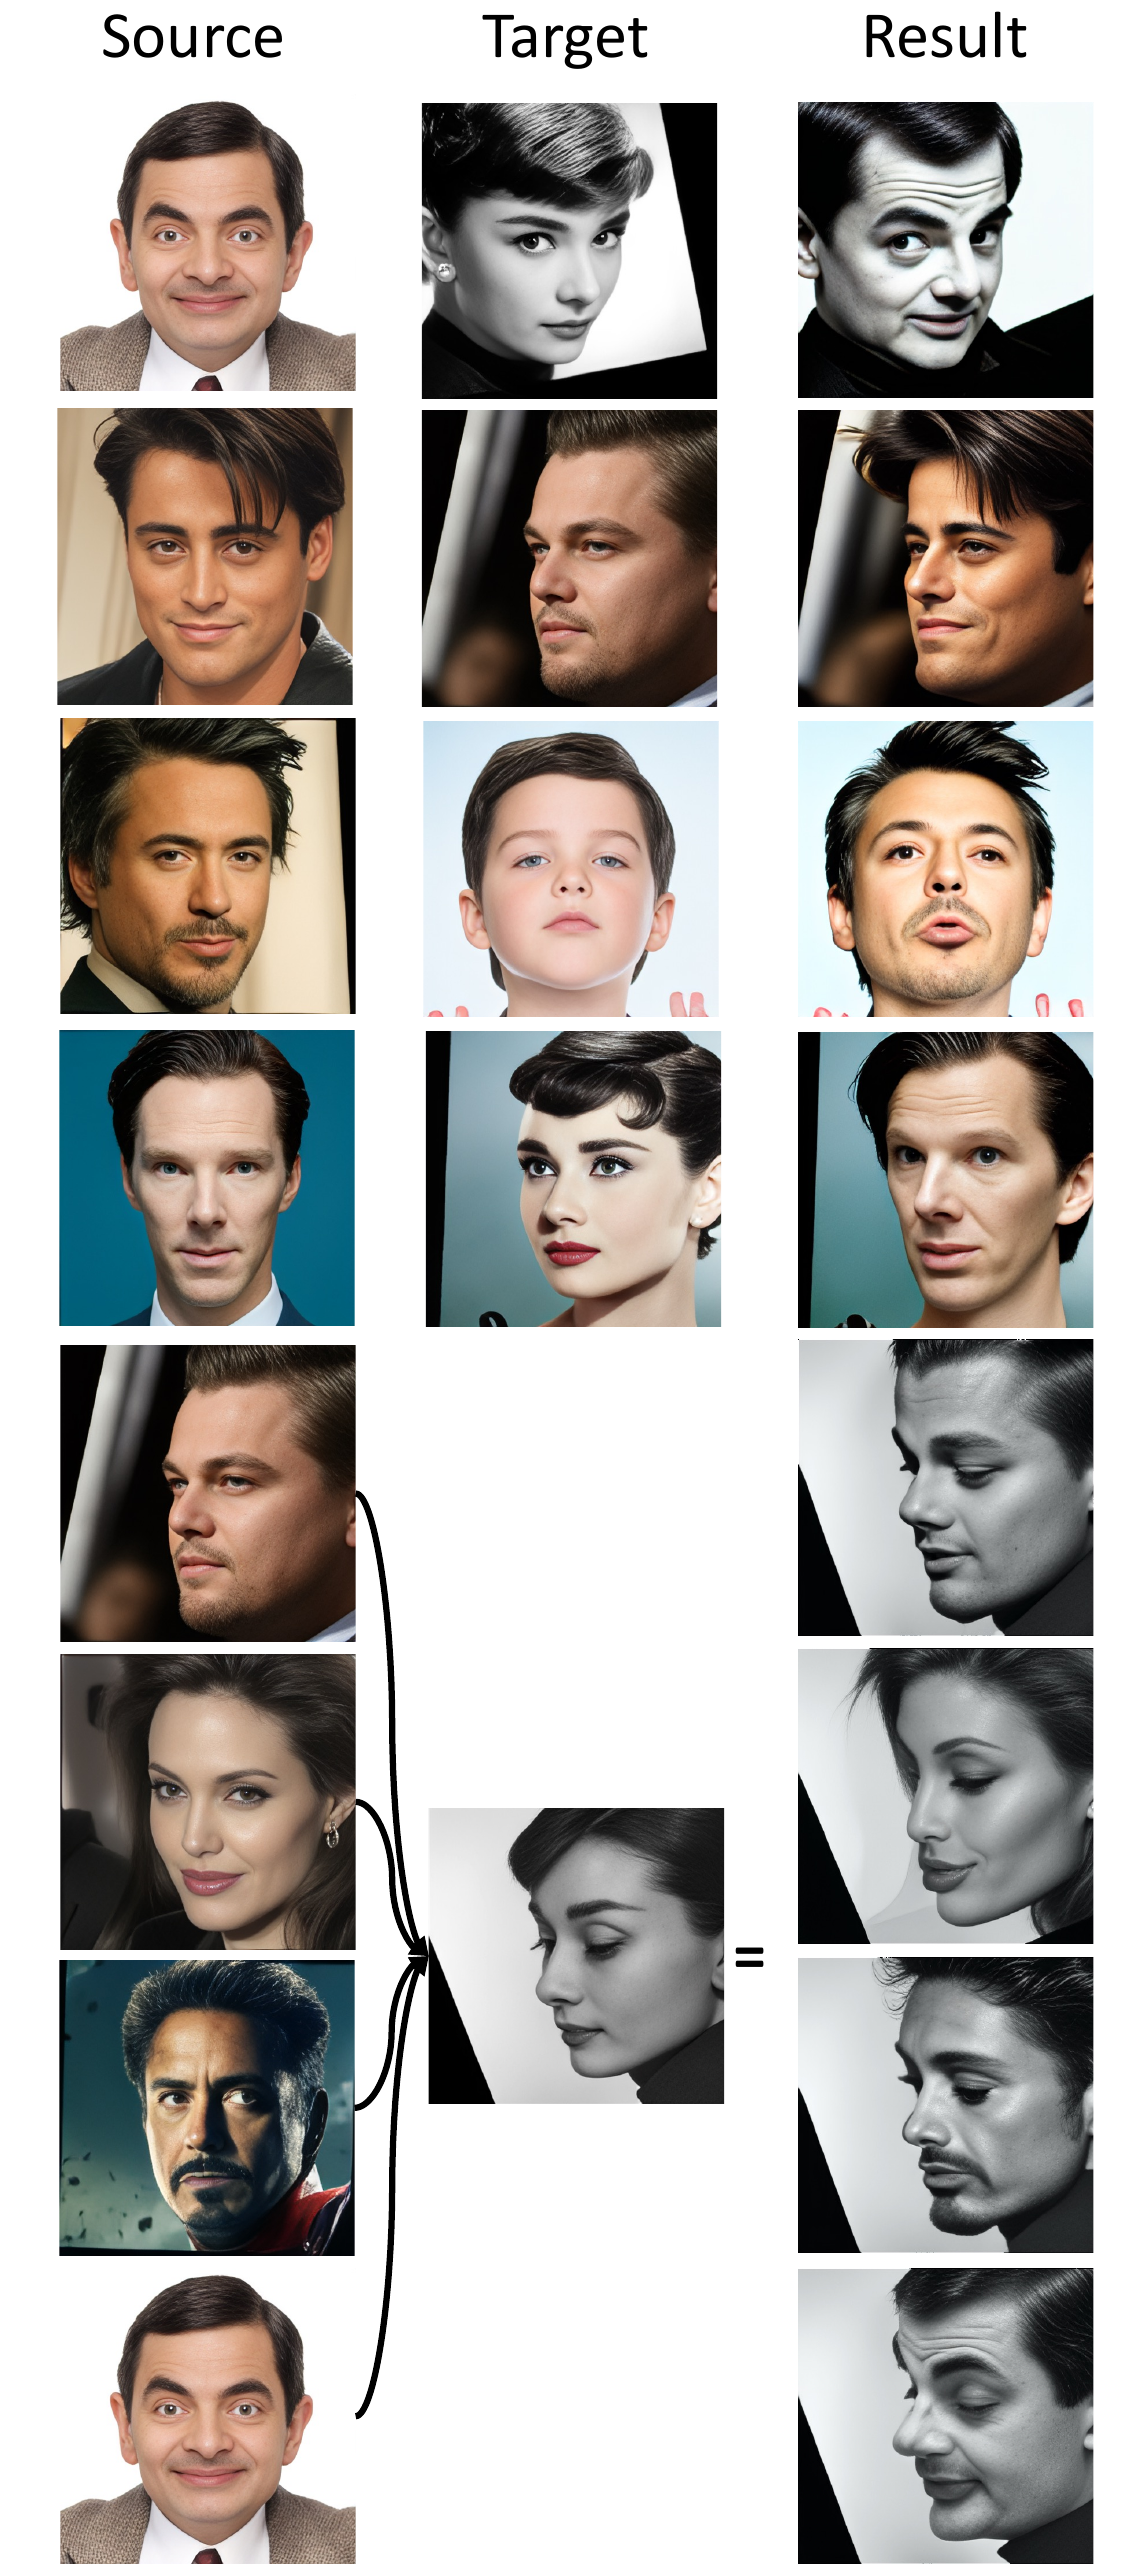}
	\vspace{2mm}
	\caption{Head Swapping in the wild.}
	\label{fig:headswapwild}
	\vspace{2em}
\end{figure} 
\begin{figure*}[h!]
	\centering
	\includegraphics[width=\linewidth]{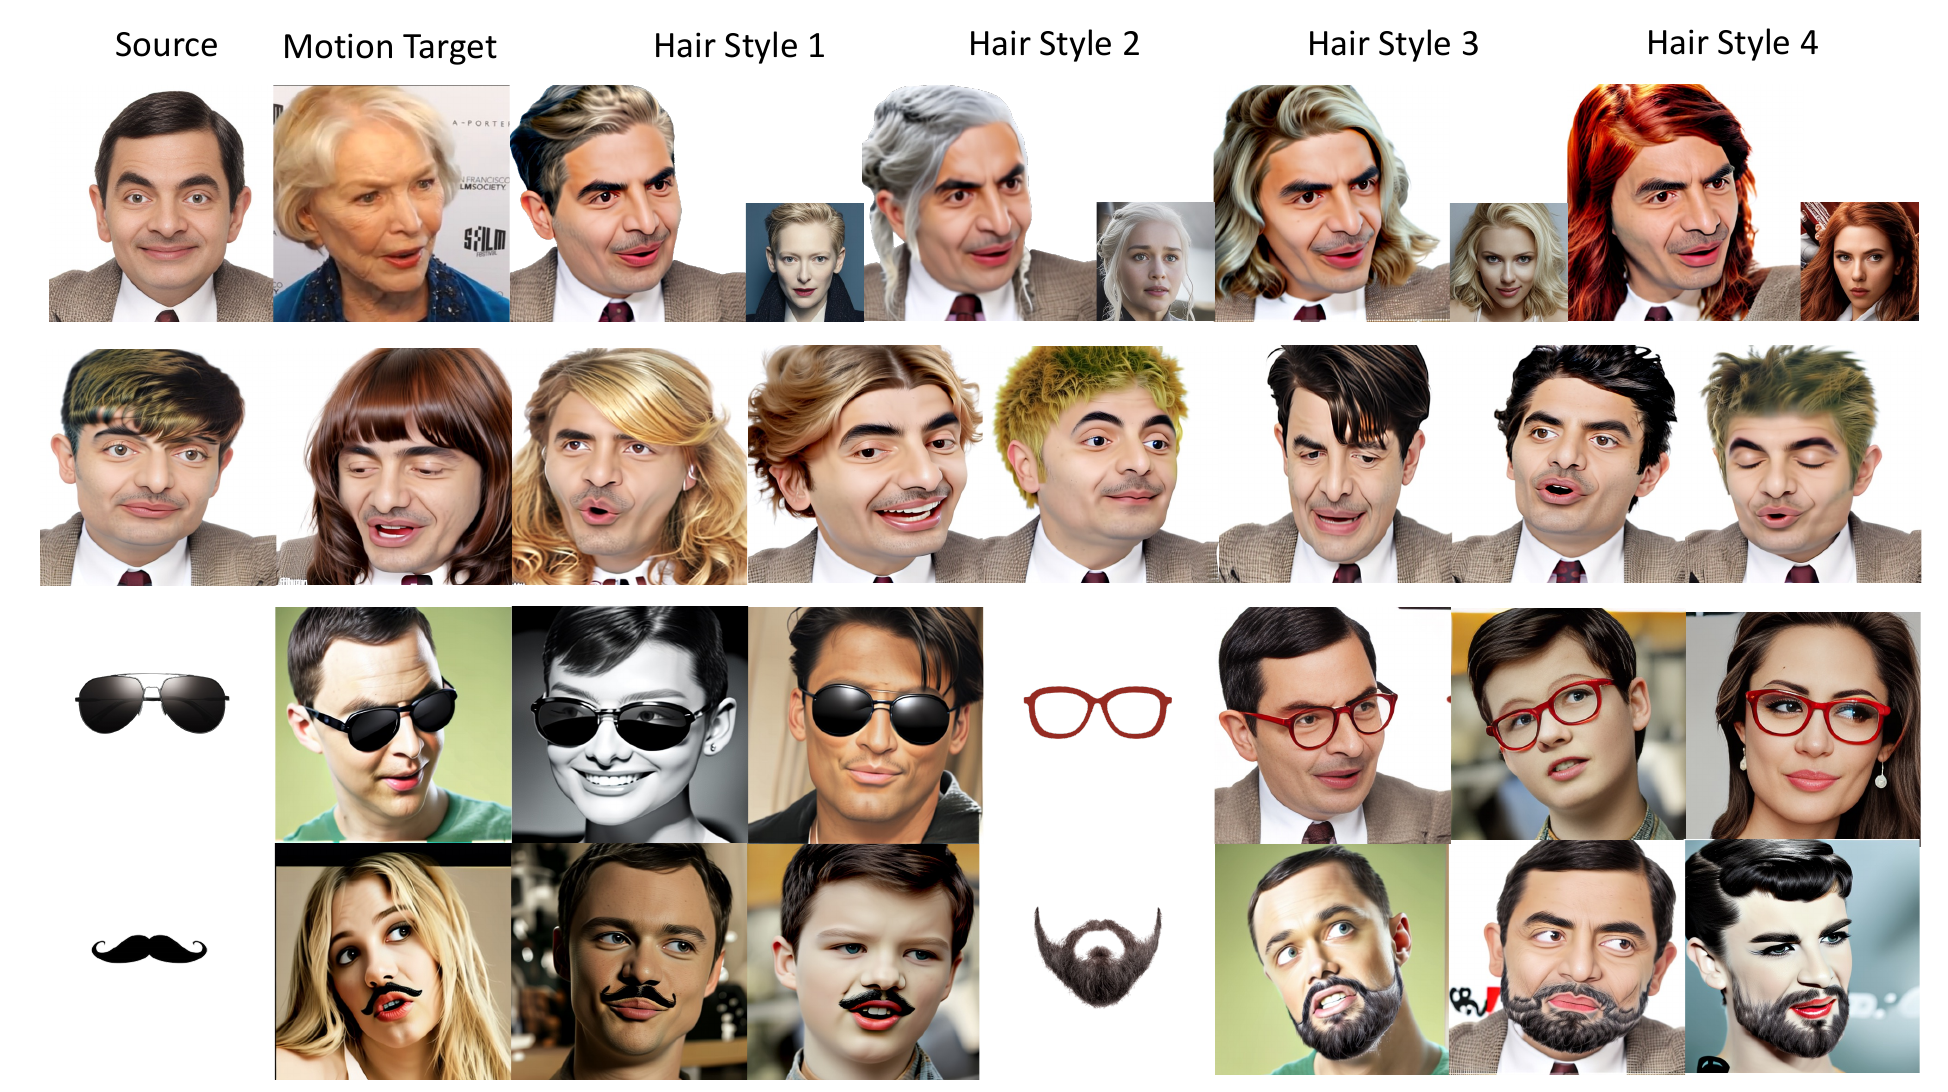}
	% \vspace{-10mm}
	\caption{Attribute Editing in the wild.}
	\label{fig:mixedit}
	% \vspace{-5em}
\end{figure*} 
